# Supplementary material for: Unlocking Generalization for Robotics via Modularity and Scale
Source: arXiv:2503.06814 source file (2025-03-10)
Supplement: Supplementary file 1 [file appendix.tex]

\input{chapters/raps/supp_text}
\clearpage

\input{chapters/psl/supp_text}
\clearpage

\input{chapters/raps/supp_text}
\clearpage

\input{chapters/psl/supp_text}
\clearpage

\clearpage

\input{chapters/nmp/supplement}
\clearpage

\input{chapters/manipgen/supplement}
\clearpage
\clearpage

\input{chapters/nmp/supplement}
\clearpage

\input{chapters/manipgen/supplement}
\clearpage
